# Supplementary material for: Empirically Analyzing Ethereum's Gas Mechanism
Source: arXiv:1905.00553 source file (2019-05-02)
Supplement: Supplementary file 1 [file appendices.tex]

\begin{appendices}
\includegraphics{../data/exec-thread-callgraph.png}
\end{appendices}
